# Supplementary material for: Fair Energy Allocation in Risk-aware Energy Communities
Source: arXiv:2303.07879 source file (2023-05-22)
Supplement: Supplementary file 1 [file Appendix.tex]

\section{Game Analysis - Proofs} \label{sec:uncoordinated_appendix}

In this section, we investigate the operational states of the distributed, uncoordinated energy source selection for both risk-conservative and risk-seeking consumers. Specifically, we study the conditions on the parameter values for the existence of dominant strategies or mixed-strategy NE under PA. To derive the NE, we recall that any mixed strategy NE $\mathbf{p^{NE}}$
%=(\mathbf{p_0^{NE}}, \mathbf{p_1^{NE}}, ..., \mathbf{p_{M-1}^{NE}})^T$, with $\mathbf{p}^{NE}_{\ell}=[p^{NE}_{RES,\ell}, p^{NE}_{nonRES,\ell}]^T$,
must fulfill


\small
\begin{equation}\label{eq:cost_equality_mixed}
\upsilon_{RES, \ell}(\mathbf{p^{NE}})= \upsilon_{nonRES, \ell}(\mathbf{p^{NE}}), ~\forall \ell \in \Theta.
\end{equation}
\normalsize

\noindent Namely, the expected costs of each pure strategy in the support of the mixed-strategy equilibrium  ($\mathcal{A}$) are equal. By substituting the expressions of \eqref{eq:RES_cost} and \eqref{eq:nonRES_cost2} in \eqref{eq:cost_equality_mixed}, we obtain that the amount of RESs allocated to $\ell \in \Theta$ at a NE should satisfy

\small
\begin{equation}\label{eq:conditionEQ_extra_demand}
rse^{PA, NE}_{\ell}(\mathbf{p^{NE}}) = \frac{\gamma-\epsilon_{\ell}\beta}{\gamma-1}E_{\ell},~ \forall \ell \in \Theta.
\end{equation}
\normalsize

\noindent Thus, when combining the Energy Source Selection Game with the PA policy, the existence of a NE is under the condition


\small
\begin{equation}\label{eq:condition_PA_NE}
rse_{\ell}^{PA}(\mathbf{p}^{NE}) =rse_{\ell}^{PA,NE}(\mathbf{p}^{NE}), \forall \ell \in \Theta. \end{equation}
\normalsize

\noindent 
Therefore, for all cases, any existing mixed-strategy NE competing probabilities, $\mathbf{p}^{NE}$, are obtained so as to satisfy the relation \eqref{eq:condition_PA_NE}. In the following we distinguish several cases based on the parameters values, namely the RES capacity, the risk aversion degrees, and the day-time energy demand levels.

\subsection{\textbf{Case $1$: The RES capacity, $\mathcal{ER}$, exceeds the maximum total demand for RES $D^{Total}$ ($\mathcal{ER} \geq D^{Total}$).}}

As the consumers have knowledge of $\mathcal{ER}$ and $D^{Total}$, it is straightforward to show that the dominant-strategy for all consumers is to select the strategy $RES$. As result, the competing probabilities that lead to equilibrium states are equal to $1$ for all consumers' types, and the expected aggregate demand for RES at NE is equal to $D^{Total}$.

In all the remaining cases, we assume that $\mathcal{ER}< D^{Total}$. Three distinct cases are defined with respect to the risk aversion degrees of the consumers and energy prices.

\subsection{\textbf{Case $2$: The risk aversion degrees for all consumers' types satisfy $1\leq \epsilon_{\ell}<\gamma/\beta$, $\forall \ell \in \Theta$.}}

We distinguish the following sub-cases with respect to the day-time energy demand levels. 

\subsubsection{\textbf{Sub-case $2(a)$: The day-time energy demand levels satisfy  $E_{\ell } \leq \mathcal{ER}\frac{(\gamma-1)}{(\gamma-\epsilon_{\ell }\beta)}$,  for all $\ell \in \Theta$}}

In this case, a mixed-strategy NE with the PA policy exists if and only if for every pair of consumers, $i,j$ with day-time energy demand levels $E_{\vartheta_i}$, $E_{\vartheta_j}$, respectively, it holds that

\small
\begin{eqnarray}\label{eq:relation_E_0_E_1_pa_ne_extra_demand}
\mathcal{ER}\frac{(\gamma-1)}{(\gamma-\epsilon_{\vartheta_i }\beta)}-E_{\vartheta_i} &=& \mathcal{ER}\frac{(\gamma-1)}{(\gamma-\epsilon_{\vartheta_j }\beta)}-E_{\vartheta_j}.
 \end{eqnarray}
\normalsize

\begin{proof}
To derive the condition \eqref{eq:relation_E_0_E_1_pa_ne_extra_demand} we first consider a consumer $i$ with type $\vartheta_i \in \Theta$ that plays $RES$. Then, we can substitute the left-hand side of \eqref{eq:condition_PA_NE} with \eqref{eq:prop_alloc_energy} where the demand for RESs is expressed as $D(\mathbf{p^{NE}}) = E_{\vartheta_i}+ \sum_{ {\ell}\in \Theta} r_{\ell}~ (N-1)~E_{\ell}~p^{NE}_{RES,\ell}$. And, by substituting the right-hand side of \eqref{eq:condition_PA_NE} with \eqref{eq:conditionEQ_extra_demand} for consumer $i$, we obtain:

\begin{small}
\begin{align}
&  \mathcal{ER}\frac{(\gamma-1)}{(\gamma-\epsilon_{\vartheta_i}\beta)}-E_{\vartheta_i}= \sum_{ {\ell}\in \Theta} r_{\ell}~ (N-1)~E_{\ell}~p^{NE}_{RES,\ell},
    \label{eq:probrelation1}
\end{align}
\end{small}

\noindent By analogy, we can re-write \eqref{eq:relation_E_0_E_1_pa_ne_extra_demand} for a consumer $j$ with type $\vartheta_j \in \Theta \setminus \{\vartheta_i\}$ that plays $RES$ as:

\begin{small}
\begin{align}
  &  \mathcal{ER}\frac{(\gamma-1)}{(\gamma-\epsilon_{\vartheta_j}\beta)}-E_{\vartheta_j}=  \sum_{ {\ell}\in \Theta} r_{\ell} ~(N-1)~E_{\ell}~ p^{NE}_{RES,\ell}.
    \label{eq:probrelation2}  
\end{align}
\end{small}

\noindent Since the right-hand sides of \eqref{eq:probrelation1}-\eqref{eq:probrelation2} are equal, the left-hand sides will be also equal and \eqref{eq:relation_E_0_E_1_pa_ne_extra_demand} derives.
\end{proof}

Under condition \eqref{eq:relation_E_0_E_1_pa_ne_extra_demand}, the competing probabilities $p^{PA,NE}_{RES,{\vartheta_i}}$ for each consumer $i$ of type $\vartheta_i \in \Theta$ that lead to equilibrium states lie in the range:


\footnotesize
\begin{align}
&  \Biggl[ \max \Biggl\{0,\frac{\mathcal{ER}\frac{(\gamma-1)}{(\gamma-\epsilon_{\vartheta_i}\beta)}-E_{\vartheta_i}-
  \sum_{ {\ell}\in \Theta \setminus \{{\vartheta_i}\}} r_{\ell} (N-1)E_{\ell}}{r_{\vartheta_i}(N-1)E_{\vartheta_i}}\Biggl\}, \nonumber \\
 &      \min\Biggl\{1,\frac{\mathcal{ER}\frac{(\gamma-1)}{(\gamma-\epsilon_{\vartheta_i}\beta)}-E_{\vartheta_i}}{r_{\vartheta_i}(N-1)E_{\vartheta_i}}\Biggl\}
    \Biggr].
    \label{eq:prop_alloc_pa_bounds_0_extra_demand}
\end{align}
\normalsize

\begin{proof}
This range is derived by taking extreme values ($0$ and $1$) of all probabilities $p^{PA,NE}_{RES,{\ell}}$ for all other consumers' types $\ell \in \Theta \setminus \vartheta_i$ in \eqref{eq:probrelation1}. Specifically, to obtain the lower (upper) bound we assign unary (zero) probabilities to all other consumers' types.
\end{proof}

Furthermore, at NE, the expected aggregate demand for RES can be expressed, for any consumers' type $\ell \in \Theta$, as:

\footnotesize
\begin{align}
& D(\mathbf{p}^{NE})= \min\Bigl\{D^{Total}, \max\Bigl\{\left[\mathcal{ER}\frac{(\gamma-1)}{(\gamma-\epsilon_{\ell}\beta)}-E_{\ell}\right]\frac{N}{(N-1)},0\Bigr\}\Bigr\}.
    \label{eq:demand1}
\end{align}
\normalsize

\begin{proof}
To derive \eqref{eq:demand1}, we multiply \eqref{eq:probrelation1} with $\frac{N}{N-1}$ and use the definition of the demand for RESs in \eqref{eq:demand}.
\end{proof}


\begin{remark}\label{rem:risk_seeking}If all consumers are risk-seeking (i.e., $\epsilon_{\vartheta_i}= 1, \forall i \in \mathcal{N}$), a NE can exist only if  $E_{0}=E_{1}=...=E_{M-1}$.%for every pair of $\vartheta_i, \vartheta_j \in \Theta$. %On the contrary, if there are risk-conservative consumers, they may need to have asymmetric energy profiles for a NE to exist.
\end{remark}

\begin{remark} \label{rem:risk_degrees_relation}
Note that condition \eqref{eq:relation_E_0_E_1_pa_ne_extra_demand} can hold, and therefore a NE can exist, only if $\epsilon_0\leq \epsilon_1 \leq..\leq \epsilon_{M-1}$. Since by assumption, $E_0\leq E_1 \leq ...\leq E_{M-1}$, this means that consumers with lower day-time energy demand levels should be less risk-averse than those with higher ones.
\end{remark}

 
\subsubsection{\textbf{Sub-case $2(b)$: The day-time energy demand levels satisfy $E_{\ell} > \mathcal{ER}\frac{(\gamma-1)}{(\gamma-\epsilon_{\ell}\beta)}$  for all $\ell \in \Theta$}} 
In this case, the dominant strategy for all consumers is to play $nonRES$.

\begin{proof}
To prove this, we show that $\upsilon_{RES, \vartheta_i}(\mathbf{p})>\upsilon_{nonRES, \vartheta_i}(\mathbf{p})$, for any consumer $i\in \mathcal{N}$ of type $\vartheta_i \in \theta$, and $\forall \mathbf{p}$. 

Firstly, let us assume that $\vartheta_i=0$ and that the allocated energy is $E'$. Then, for a large population, we have $\upsilon_{RES, 0}(\mathbf{p})= E'  \cdot c_{RES}+(E_0-E')\cdot \gamma \cdot  c_{RES}$ and
$\upsilon_{nonRES, 0}(\mathbf{p})= \epsilon_0 \cdot E_0 \cdot \beta \cdot c_{RES}$. The inequality $\upsilon_{RES,0}(\mathbf{p})>\upsilon_{nonRES, 0}(\mathbf{p})$ is then equivalent to the inequality $E_0 >E' \frac{(\gamma-1)}{(\gamma-\epsilon_0\beta)}$, which is true by assumption, since $E'<\mathcal{ER}$.

By analogy, the same can be shown for every $\vartheta_i\in \Theta$.
\end{proof}


As result, the competing probabilities that lead to equilibrium states are equal to $0$ for all consumers' types $\vartheta_i\in \Theta$, and the expected aggregate demand for RES at NE is equal to $0$.

\subsubsection{\textbf{Sub-case $2(c)$: There exist two distinct subsets of consumers' types, $\Sigma_1 , \Sigma_2 \subset \Theta$, such that $\{E_{\ell} > \mathcal{ER}\frac{(\gamma-1)}{(\gamma-\epsilon_{\ell}\beta)}, ~\forall \ell \in \Sigma_1\}$ and $\{E_{\ell} \leq \mathcal{ER}\frac{(\gamma-1)}{(\gamma-\epsilon_{\ell}\beta)}, ~ \forall \ell \in \Sigma_2\}$}}

For consumers whose types are in the set $\Sigma_1$, the dominant strategy is to play $nonRES$. 
\begin{proof}
By analogy, this proof can directly be derived from the proof in Sub-case $2(b)$, where the set of all consumers' types $\Theta$ is replaced by the set $\Sigma_1$.
\end{proof}
For consumers whose types are in the set $\Sigma_2$, the mixed strategy NE is determined under the condition of \eqref{eq:relation_E_0_E_1_pa_ne_extra_demand}. 
\begin{proof}
By analogy, this proof can directly be derived from the proof in Sub-case $2(a)$, where the set of all consumers' types $\Theta$ is replaced by the set $\Sigma_2$.
\end{proof}

Additionally, for consumers whose types are in $\Sigma_1$, the competing probabilities at NE are equal to $0$, whereas, for consumers $i$ of type $\vartheta_i \in \Sigma_2$, the competing probabilities that lead to a NE states lie in the range:

\footnotesize
\begin{align}
&  \Biggl[ \max \biggl\{0,\frac{\mathcal{ER}\frac{(\gamma-1)}{(\gamma-\epsilon_{\vartheta_i}\beta)}-E_{\vartheta_i}-
  \sum_{\ell \in \Sigma_2 \setminus \{\vartheta_i\}} r_{\ell} (N-1)E_{\ell}}{r_{\vartheta_i}(N-1)E_{\vartheta_i}}\Biggr\}, \nonumber \\
    & \min \Biggl\{1,\frac{\mathcal{ER}\frac{(\gamma-1)}{(\gamma-\epsilon_{\vartheta_i}\beta)}-E_{\vartheta_i}}{r_{\vartheta_i}(N-1)E_{\vartheta_i}}\Biggr\}
    \Biggr].
    \label{eq:prop_alloc_pa_bounds_0_extra_demandnew}
\end{align}
\normalsize

\begin{proof}
By analogy, this result is obtained similarly to Eq.  \eqref{eq:prop_alloc_pa_bounds_0_extra_demand} in Sub-case $2(a)$ where the set of all consumers' types $\theta$ is replaced by the set of consumers' types $\Sigma_2$.
\end{proof}

Finally, the aggregate demand for RESs in $\Sigma_2$ is equal to $0$, and the total aggregate demand for RESs can be expressed as

\footnotesize
\begin{align}
& D(\mathbf{p}^{NE})= \min\Bigl\{ D^{Total}_{\Sigma_2} , \max\Bigl\{\left[\mathcal{ER}\frac{(\gamma-1)}{(\gamma-\epsilon_{\ell}\beta)}-E_{\ell}\right]\frac{N}{(N-1)},0\Bigr\}\Bigr\},
    \label{eq:demand1_2c}
\end{align}
\normalsize

\noindent where $D^{Total}_{\Sigma_2} = N  \sum_{\tilde{\ell } \in \Sigma_2} r_{\tilde{\ell }  }E_{\tilde{\ell } }$ is the maximum demand for RESs of the consumers whose types are in $\Sigma_2$.

\begin{proof}
By analogy with subcase $2(a)$, we derive \eqref{eq:demand1_2c} similarly to \eqref{eq:demand1}, in which $D^{Total}$ is replaced by $D^{Total}_{\Sigma_2}$, the maximum demand for RESs of the consumers whose types are in $\Sigma_2$.
\end{proof}

\begin{remark}
We note that Remark \ref{rem:risk_degrees_relation} now holds for all consumers' types in $\Sigma_2$.
\end{remark}

\subsection{\textbf{Case $3$: The risk aversion degrees satisfy $\epsilon_{\ell} \geq \gamma/\beta$, $\forall \ell \in \Theta$.}}

In this case, the dominant strategy for all consumers is to play $RES$. 

\begin{proof}
To prove this, we show that $\upsilon_{RES, \vartheta_i}(\mathbf{p})<\upsilon_{nonRES, \vartheta_i}(\mathbf{p})$, $\forall \mathbf{p},~ \forall i\in \mathcal{N}$. 

Firstly, we assume that $\vartheta_i=0$ and that the allocated energy is $E'$. Then, the inequality $\upsilon_{RES,0}(\mathbf{p})<\upsilon_{nonRES, 0}(\mathbf{p})$ is equivalent to the inequality $E_0 >E' \frac{(\gamma-1)}{(\gamma-\epsilon_0\beta)}$. This is true by assumption, since $(\gamma-\epsilon_0\beta)\leq 0$ in this case.

By analogy, similar inequality can be derived for all consumers $i \in \mathcal{N}$ of type $\vartheta_i \in \Theta$.
\end{proof}

Therefore, the competing probabilities that lead to equilibrium states are equal to $1$ for all consumers' types, and the aggregate demand for RESs at NE is equal to $D^{Total}$.

\subsection{\textbf{Case $4$: There exist two distinct subsets of consumers' types, $\Sigma_1 , \Sigma_2 \subset \Theta$, such that $\Bigl\{\epsilon_{\ell} \geq \gamma/\beta, ~ \forall \ell \in \Sigma_1 \Bigr\}$, and $\Bigl\{\epsilon_{\ell} < \gamma/\beta,~\forall \ell \in \Sigma_2 \Bigr\}$.}} 

By analogy with Case $3$, for the consumers whose type is in the set $\Sigma_1$, the dominant strategy is to compete for RESs.
By analogy with Case $2$, for the consumers whose type is in the set $\Sigma_2$, three sub-cases  $4(a)-(c)$ are defined with respect to their day-time energy demand levels. All the conditions derived in Case $2$ can straightforwardly be extended to the consumers' types in $\Sigma_2$, considering that all consumers in $\Sigma_1$ play $RES$. To do so, we adjust the available RES capacity by subtracting to it the aggregate demand for RESs from consumers' types in $\Sigma_1$. For the sake of concision we do not detail these conditions.


\begin{table}[ht!]\label{table:cases}
\begin{minipage}{\textwidth}
\centering
\begin{tabular}{p{.065\textwidth}p{.21\textwidth}p{.21\textwidth}p{.21\textwidth}p{.21\textwidth}}
\hline
                                 &  &              & \textbf{Proportional allocation}          & \textbf{Equal sharing}            \\ \hline
\textbf{Case 1:}                  &  $\mathcal{ER} \geq D^{Total}$ & \textbf{}    &     Dominant-strategy for all consumers to play $RES$    \par \      &  Dominant-strategy for all consumers to play $RES$     \par \                                  \\
\multirow{3}{=}{\textbf{Case 2:}} &  \multirow{3}{=}{$\mathcal{ER} < D^{Total}$, and $1\leq \epsilon_{\vartheta_i}<\gamma/\beta$, $\forall i\in \mathcal{N}$} & \textbf{(a)}  $E_{\vartheta_i } \leq \mathcal{ER}\frac{(\gamma-1)}{(\gamma-\epsilon_{\vartheta_i }\beta)}$, $ \forall \vartheta_i \in \Theta$ &   Mixed-strategy NE under condition \eqref{eq:relation_E_0_E_1_pa_ne_extra_demand}   \par \                 &       Mixed-strategy NE under condition \eqref{eq:relation_E_0_E_1_es_ne_extra_demand}   \par \                                    \\
                                 &  & \textbf{(b)} $E_{\vartheta_i} > \mathcal{ER}\frac{(\gamma-1)}{(\gamma-\epsilon_{\vartheta_i}\beta)}$, $ \forall \vartheta_i \in \Theta$ &   Dominant-strategy for all consumers to play $nonRES$    \par \   &   Dominant-strategy for all consumers to play $nonRES$    \par \                            \\
                                 &  & \textbf{(c)} $\exists \ \vartheta_i \in \Sigma_1$, s.t. $E_{\vartheta_i} > \mathcal{ER}\frac{(\gamma-1)}{(\gamma-\epsilon_{\vartheta_i}\beta)}$, and $\exists \ \vartheta j \in \Sigma_2$, s.t. $E_{\vartheta_j} \leq \mathcal{ER}\frac{(\gamma-1)}{(\gamma-\epsilon_{\vartheta_j}\beta)}$ &      Dominant-strategy for all consumers types  $\vartheta_i \in \Sigma_1$ to play $nonRES$, mixed-strategy NE for consumer types $\vartheta_j \in \Sigma_2$ under condition \eqref{eq:relation_E_0_E_1_pa_ne_extra_demand} \par \                   &     Dominant-strategy for all consumers types  $\vartheta_i \in \Sigma_1$ to play $nonRES$, mixed-strategy NE for consumer types $\vartheta_j \in \Sigma_2$ under condition \eqref{eq:relation_E_0_E_1_es_ne_extra_demand}   \par \                                  \\
\textbf{Case 3:}    &               $\mathcal{ER}<D^{Total}$, and $\epsilon_{\vartheta_i} \geq \gamma/\beta$, $\forall i\in \mathcal{N}$      &  \textbf{}   & Dominant-strategy for all consumers to play $RES$ \par \   &     Dominant-strategy for all consumers to play $RES$    \par \                                \\
\textbf{Case 4:}                  & $\mathcal{ER}<D^{Total}$,  $\exists \ \vartheta_i \in \Sigma_1$, s.t. $\epsilon_{\vartheta_i} \geq \gamma/\beta$, and $\exists \ \vartheta_j \in \Sigma_2$, s.t. $\epsilon_{\vartheta_j} < \gamma/\beta$ & \textbf{}    &    Dominant strategy for all consumer types $\vartheta_i \in \Sigma_1$ to play $RES$ , mixed-strategy NE for consumer types $\vartheta_j \in \Sigma_2$ under condition \eqref{eq:relation_E_0_E_1_pa_ne_extra_demand} \par \ &   Dominant strategy for all consumer types $\vartheta_i \in \Sigma_1$ to play $RES$ , mixed-strategy NE for consumer types $\vartheta_j \in \Sigma_2$ under condition \eqref{eq:relation_E_0_E_1_es_ne_extra_demand}   \par    \       \\ \hline                     
\end{tabular}
\caption{Analysis of uncoordinated mechanism}
\end{minipage}
\end{table}



\section{Centralized Energy Source Allocation Mechanism - Proofs}\label{sec:coordinated}

In this section, we study the centralized mechanism that allocates the different energy sources to the $N$ consumers of the micro-grid.

\subsection{Optimization Problem Formulation}

In practice, in the centralized mechanism, all consumers, $i \in \mathcal{N}$ with type $\vartheta_i \in \Theta$ issue energy demand requests $E_{\vartheta_i}$ to a central micro-grid operator that optimally processes their requests and allocates resources. 
%Therefore, the aggregate amount of day-time loads is equal to $D^{Total}$. 
The centralized mechanism aims at minimizing the social cost of all consumers by optimally allocating this demand between the night and day. 

In practice, this coordinator's energy source allocation policy is represented as an optimization problem which aims at minimizing the social cost  $C(\mathbf{p}^{OPT})$ for all the consumers, defined as:

\begin{small}
\begin{align}
C(\mathbf{p}^{OPT}) & = \min\Bigl\{ \mathcal{ER}, N \sum_{{\ell} \in \Theta} r_{\ell} p_{RES,{\ell}}^{OPT}  E_{\ell}\Bigr\}  c_{RES} \nonumber \\ & + \max \Bigl\{ 0,N \sum_{{\ell} \in \Theta} r_{\ell} p_{RES,{\ell}}^{OPT}  E_{\ell}- \mathcal{ER}\Bigr\}  c_{nonRES}\nonumber \\
& + N  \sum_{{\ell} \in \Theta} r_{{\ell} }p^{OPT}_{nonRES,{\ell}}\varepsilon_{{\ell} }E_{{\ell}} c_{nonRES,N},
 \label{eq:social_cost_x_opt}
 \end{align}
\end{small}

\noindent where, the decision variables of the centralized mechanism are the optimal probability distributions ($p^{OPT}_{RES,\vartheta_i}$, $p^{OPT}_{nonRES,\vartheta_i}$), which represent the optimal probability that consumer $i$ with type $\vartheta_i$ engages its load during day, or during the night, respectively, for all consumers $i \in \mathcal{N}$. \footnote{The vector $\mathbf{p^{OPT}}$ is defined similarly to $\mathbf{p^{NE}}$.}

%where $N  \sum_{{\ell}\in \Theta} r_{\ell} p_{RES,{\ell}}^{OPT}  E_{\ell} $ represents the total RES production allocated in the day-zone, and $N  \sum_{{\ell} \in \Theta} r_{{\ell} }p^{OPT}_{nonRES,{\ell}}\varepsilon_{{\ell} }E_{{\ell}}$ represents the total nonRES production allocated in the night-zone. %The first summand refers to the consumers who are served by low-cost RES capacity during the day. The second summand is for the consumers who are served $nonRES$ duing the night-zone. 
%In other words, the part of the optimal social cost that corresponds to the day-zone peak-load production will be zero. %The social costs under the PA and ES policies are defined similarly to Eqs. \eqref{eq:social_cost_pa_extra_demand} and \eqref{eq:social_cost_es}, respectively. 


The optimal solutions of this centralized mechanism will provide a benchmark against which to evaluate the side-effects that stem from the distributed, uncoordinated energy source selection, in terms of social cost. In the following, we provide insights and analytical formulations for the energy allocation, the social cost and the PoA under the PA mechanism. For the ES mechanism, the centralized decisions for minimizing the social cost are harder to derive analytically and we will present numerical evaluations in Section \ref{sec:eval} using software optimization tools, namely, Mathematica and MATLAB.

\subsection{Optimal Centralized Solutions}

%%%%%%%%% define these costs under each allocation policy!!!????
We derive the properties of the solution provided by the centralized mechanism, $\mathbf{p^{OPT}}$, in four cases, identical to the ones defined in Section \ref{sec:uncoordinated_extra_demand}.
 
\subsubsection{\textbf{Case $1$: The RES capacity exceeds the maximum consumer demand}}

In this trivial case, the social cost reduces to:

\begin{small}
\begin{align}
C(\mathbf{p}^{OPT}) & = N \sum_{{\ell} \in \Theta} r_{\ell} p_{RES,{\ell}}^{OPT}  E_{\ell}   c_{RES}  \nonumber \\
& + N  \sum_{{\ell} \in \Theta} r_{{\ell} }p^{OPT}_{nonRES,{\ell}}\varepsilon_{{\ell} }E_{{\ell}} c_{nonRES,N},
 \label{eq:social_cost_x_opt_case1}
 \end{align}
\end{small}

\noindent and the optimal solution of the centralized mechanism is $p^{OPT}_{RES,\vartheta_i}=1$, and $p^{OPT}_{nonRES,\vartheta_i}=0$, $\forall \vartheta_i \in \Theta$.

In all other cases considered, the RES capacity is lower than the maximum consumer demand.

\subsubsection{\textbf{Case $2$: The risk-aversion degrees of all consumers' types are lower than $\gamma/\beta$}}

In this case, the optimal probability distributions are shaped so that the total renewable energy capacity is utilized and the remaining demand is shifted to the night zone. Specifically, the social cost reduces to:

\begin{small}
\begin{align}
C(\mathbf{p}^{OPT}) &=  \mathcal{ER} \cdot c_{RES}   \nonumber \\
&+N \left[ \sum_{{\ell} \in \Theta} r_{\ell }p^{OPT}_{nonRES,{\ell}}\varepsilon_{{\ell} }E_{{\ell}}\right] c_{nonRES,N}
 \label{eq:social_cost_pa_extra_demand_2}
 \end{align}
\end{small}

\noindent Therefore, to derive $\mathbf{p^{OPT}}$ the centralized mechanism needs to minimize the night-rate cost, under the constraint that the total energy demand for RES equals the RES capacity: 
%\vspace{-5pt}
\small
\begin{align}
N \sum_{{\ell} \in \Theta}r_{{\ell}} E_{{\ell}}p^{OPT}_{RES,{\ell}}=\mathcal{ER}.
\label{eq:optimal}
\end{align}
\normalsize

\noindent This can be done using a software optimization tool such as Mathematica or MATLAB. And we show that the optimal competing probabilities $p^{OPT}_{RES,\vartheta_i}$ for all $ \vartheta_i \in \Theta$ lie in the range:

\footnotesize
\begin{align}
 \hspace{-5pt} 
 \Biggl[max\left\{0,\frac{\left[\mathcal{ER} -\sum_{{\ell} \in \Theta \setminus \{\vartheta_i\}}r_{{\ell}}N E_{{\ell}}\right]}{r_{\vartheta_i}N E_{\vartheta_i}}\right\},
   %\notag\\
    % min\left(1,\mathcal{ER} \frac{1}{rNE_0}\right)
    min\left\{1,\frac{\mathcal{ER}}{r_{\vartheta_i}N E_{\vartheta_i}}\right\}
    \Biggr].
    \label{eq:prop_alloc_opt_bounds_0}
\end{align}
\normalsize

\begin{proof}
The lower bound of the range derives using Eq. \eqref{eq:optimal} and by considering that for all consumers $j\in \mathcal{N}\setminus \{i\}$, $p^{OPT}_{RES,\vartheta_j}=1$. The upper bound derives in a similar fashion but by considering that for all $j\in \mathcal{N}\setminus \{i\}$, $p^{OPT}_{RES,\vartheta_j}=0$.
\end{proof}

%Because the risk-aversion degrees are all the same, the night-rate social cost is constant and equal to 
%$\epsilon' N \sum_{{\ell} \in \Theta}r_{\ell}E_{\ell}p^{OPT}_{nonRES,\ell} c_{nonRES,N}=\epsilon'  ( N\sum_{{\ell} \in \Theta}r_{{\ell}}E_{{\ell}}- \mathcal{ER}) c_{nonRES,N}$. Thus, the optimal cost is equal to $$C(\mathbf{p}^{OPT})=\mathcal{ER}c_{RES}+ \epsilon'  ( N\sum_{{\ell}\in \Theta}r_{{\ell}}E_{{\ell}}- \mathcal{ER}).$$

%\textbf{Case $3$.} %, which is less than $\gamma/\beta$, %depart in their policy in adjusting their demand level to the estimated risk of an action, 

%Due to the fact that the RES demand should match the RES capacity as in Case $2$,  the probabilities, $p^{OPT}_{RES,\vartheta_i} $, lie in the ranges given in (\ref{eq:prop_alloc_opt_bounds_0}). The night-rate social cost is given by $Nc_{nonRES,N} \sum_{{\ell} \in \Theta}\epsilon_{{\ell}}r_{{\ell}}E_{{\ell}}(1-p^{OPT}_{RES,{\ell}}) $. In this case, in order to obtain the optimal social cost, we need to minimize the night-rate cost under the constraint of Eq. \eqref{eq:optimal}, using a software optimization tool such as Mathematica or MATLAB. 


%Therefore, it is minimized when consumers with energy profiles $\vartheta_j \in \Theta$, corresponding to higher values of $\epsilon_{\vartheta_j}r_{\vartheta_j}E_{\vartheta_j}$ are assigned lower values of $p^{OPT}_{nonRES,\vartheta_j} $ and thus higher values of $p^{OPT}_{RES,\vartheta_j} $ (i.e., they are prioritized for RES). In addition, due to the fact that the RES demand should match its supply as in Case $2$,  the probabilities lie in the ranges given in (\ref{eq:prop_alloc_opt_bounds_0}). 


%We can obtain the expression of the optimal social cost in the simple scenario of two energy profiles. The expected cost at night-rate is $(\epsilon_0 r_0 N p^{OPT}_{nonRES,0}E_0+\epsilon_1 r_1 N p^{OPT}_{nonRES,1} E_1) c_{nonRES,N}$. Let us assume that $\epsilon_0> \epsilon_1$, then we can write $\epsilon_0= \epsilon_0'+\epsilon_1$, with $\epsilon_0'>0$. Thus, the expected cost at night-rate becomes $(\epsilon_0' r_0N p^{OPT}_{nonRES,0}E_0+\epsilon_1 (r_0 N E_0+r_1 N E_1- \mathcal{ER}) ) c_{nonRES,N}$. The only controllable term is $\epsilon_0' r_0 N p^{OPT}_{nonRES,0}E_0$ that is minimized when $ p^{OPT}_{nonRES,0}$ is minimized, i.e., when its complementary $ p^{OPT}_{RES,0}$ is maximized. Since $p^{OPT}_{RES,0}$ lie in the range given in (\ref{eq:prop_alloc_opt_bounds_0}), its optimal value will be $min\left\{1,\frac{\mathcal{ER}}{r_{\vartheta_i}N E_{\vartheta_i}}\right\}$. Having this value allows us to compute the optimal social cost. %Note that the expected cost due to use of RES will be always equal to $c_{RES} \mathcal{ER}$.


\subsubsection{\textbf{Case $3$: The risk-aversion degrees of all consumers' types are greater than $ \gamma/\beta$}}

In this case, the optimal centralized mechanism directs all consumers to play $RES$, i.e., $p^{OPT}_{RES,\vartheta_i}=1$ $\forall \vartheta_i \in \Theta$. This result is derived in a similar fashion with the result of Case $3$ in Section \ref{sec:uncoordinated_extra_demand}.
 
\subsubsection{\textbf{Case $4$: The risk aversion degrees of certain consumers' types are lower than $ \gamma/\beta$, while others are greater than $ \gamma/\beta$]}}

Then, it is an optimal solution for all consumers whose types are in the set $\Sigma_1$ to play $RES$, i.e., $p^{OPT}_{RES,\vartheta_i}=1$ $\forall \vartheta_i \in \Sigma_1$. 
Furthermore, the social cost of the consumers whose types are in $\Sigma_2$ can be expressed as: 

\begin{small}
\begin{align}
C_{\Sigma_2}(\mathbf{p}^{OPT}) &=  (\mathcal{ER} - \sum_{\ell \in \Sigma_1} r_\ell N E_\ell )\cdot c_{RES}   \nonumber \\
&+N \left[ \sum_{{\ell} \in \Theta} r_{\ell }p^{OPT}_{nonRES,{\ell}}\varepsilon_{{\ell} }E_{{\ell}}\right] c_{nonRES,N}
 \label{eq:social_cost_pa_extra_demand_2}
 \end{align}
\end{small}

\noindent where $ \mathcal{ER} - \sum_{\ell \in \Sigma_1} r_\ell N E_\ell $ represents the remaining available RES capacity, i.e., the available RES capacity minus the aggregate demand of consumers whose types are in $\Sigma_1$, who all play $RES$. Therefore, the probability that consumers whose type is in the set $\Sigma_2$ play $RES$ is optimized to minimize their night-time cost, while ensuring that they totally utilize the remaining RES capacity, such that:


\small
\begin{align}
N \sum_{{\ell} \in \Theta}r_{{\ell}} E_{{\ell}}p^{OPT}_{RES,{\ell}}=\mathcal{ER} - \sum_{\ell \in \Sigma_1} r_\ell N E_\ell.
\label{eq:optimal}
\end{align}
\normalsize

This centralized problem can be solved using a software optimization tool. And, we show that the optimal competing probabilities $p^{OPT}_{RES,\vartheta_i}$ for all $ \vartheta_i \in \Sigma_2$ lie in the range:

\footnotesize
\begin{align}
&\Biggl[\max\left\{0,\frac{\mathcal{ER}-\sum_{\ell \in \Theta \setminus \{\vartheta_i\}}r_{\ell}N E_{\ell}}{r_{\vartheta_i}N E_{\vartheta_i}}\right\}, \nonumber \\ & \min\left\{1,\frac{\mathcal{ER}-\sum_{ \ell \in \Sigma_1}r_{\ell}N E_{\ell}}{r_{\vartheta_i}N E_{\vartheta_i}}\right\}  \Biggr].
\label{eq:prop_alloc_opt_p_cond}
\end{align}
\normalsize

\noindent By analogy with Case $2$, this range is derived similarly to the one defined in \eqref{eq:prop_alloc_opt_bounds_0}.

\subsection{PoA}

The (in)efficiency of equilibrium strategies in the decentralized, uncoordinated mechanism is quantified by the Price of Anarchy (PoA) \cite{Koutsoupias09}. The PoA is expressed as the ratio of the worst case social cost among all mixed strategy NE, denoted as $C^{PA,NE}_w$, over the optimal minimum social cost of the centralized mechanism, denoted as $C(\mathbf{p^{OPT^*}})$, such that:

%\vspace{-5pt}
\small
\begin{align}
 \hspace{-5pt} \textit{PoA}^{PA}  = \frac{C^{PA,NE}_w}{C(\mathbf{p^{OPT^*}})}.
\label{eq:poa_pa}
\end{align}
\normalsize

First observe that $C(\mathbf{p^{OPT^*}})$ is uniquely determined for each particular case. Now, in order to obtain $C^{PA,NE}_w$ when there exist multiple possible NE (e.g., in Cases $2$ and $4$), we can solve a simple optimization problem to minimize the social cost $C^{PA,NE}(\mathbf{p^{PA,NE}})$ with respect to $\mathbf{p^{PA,NE}}$ and subject to the corresponding probability constraints defined in Section \ref{sec:uncoordinated_extra_demand} using a software optimization tool. Importantly, for the uncoordinated energy selection game under PA, minimizing $C^{PA,NE}(\mathbf{p^{PA,NE}})$ is equivalent to minimizing the night-time cost. %The last observation is the fact that the demand $D^{PA,NE}$ is constant with respect to $\mathbf{p^{PA,NE}}$. Also, in the special case of the risk-seeking consumers, from Eq. \eqref{eq:social_cost_pa_sc}, the social cost is constant with respect to the probabilities $\mathbf{p^{PA,NE}}$ for each case of energy profile values. Thus, $C^{PA,NE}_w$ is given by Eq. \eqref{eq:social_cost_pa_sc}.

%$2$. If having risk-conservative consumers, there exist multiple possible equilibria in the sub-cases 2(a) and 2(c) as well as in case 4. Of course, the multiple combinations of probabilities can lead to NE with possibly different social cost values. Based on the Remark \ref{rem:risk_degrees_relation}, the existence of NE is possible if consumers with lower energy demands have lower risk aversion degrees. Thus, the night cost is minimized if the optimal probabilities for RES take lower values for consumers with lower energy demands. 

\subsection{Coordinated energy allocation solutions}


The KKT conditions of the optimization problem \eqref{} are formulated as:


where $\mu$ represents the optimal dual variable associated with \eqref{eq:opt_S2_3}. 

It results that:
\begin{enumerate}
    \item for all $\ell \in Sigma_2$ s.t. $1 \leq \varepsilon_\ell < \dfrac{\gamma - \mu}{\beta}$, $p^{OPT}_{RES,\ell}=0$,
    \item for all $\ell \in Sigma_2$ s.t. $ \varepsilon_\ell = \dfrac{\gamma - \mu}{\beta}$, $0<p^{OPT}_{RES,\ell}<1$,
    \item for all $\ell \in Sigma_2$ s.t. $ \dfrac{\gamma}{\beta} > \varepsilon_\ell > \dfrac{\gamma - \mu}{\beta}$, $p^{OPT}_{RES,\ell}=1$.
\end{enumerate}
This means that the consumer types are fully dispatched during the day in order of the largest risk aversion degree (i.e. lowest day-time consumption compared to night-time consumption), until constraint \eqref{eq:opt_S2_3} is satisfied. 
